# Supplementary material for: Unsupervised Calibration under Covariate Shift
Source: arXiv:2006.16405 source file (2020-06-29)
Supplement: Supplementary file 1 [file supplementary.tex]

\section*{Supplementary}

We make use of the supplementary to provide additional experimental details (all in tables below) and discuss various) hyper-parameter selection details. 
%\subsection{Regularization in Platt}

\subsection{Additional results for importance weighted calibrator}

Similar to experiments using CDAN in the paper, we train all the classifiers using another domain adapted technique DANN (cite). We use the codes provided by CDAN authors for the same. CDAN is known to perform worse than DANN because of misalignment in source and target. Hence we expect the importance weight estimation to perform badly compared to CDAN. We notice that the transfer directions which perform well in DANN are a subset of the transfer directions which perform well in CDAN. Also we notice the the weighted estimator variance increases considerably and also the weighted calibrators performance is much worse than weighted calibrator in some cases, we attribute this is the fact that DANN inherently doesnt not ensure the alignment of features and hence produce poor feature alignment in between source and target. This can be controlled by using flattening and clipping. But we do not have labeled validation data on the target to tune these parameters.

 \begin{table}
\setlength\tabcolsep{2.5pt}
   \begin{tabularx}{0.4\linewidth}{@{} l l l @{}}
    \toprule
    Method&U$\rightarrow$M&M$\rightarrow$U\\
    \midrule
    unweighted   & 0.338          & 0.249 \\
Weighted     & \textbf{0.122} & 0.647 \\
Using target & 0.037          & 0.048 \\ \hline \hline
unweighted   & 0.171          & 0.372 \\
Weighted     & \textbf{0.068} & 0.525 \\
Using target & 0.1            & 0.183 \\
    \bottomrule
    \end{tabularx}
 \vspace{-0.1in}
\caption{mnist-usps, domain adapted using using DANN. ECE scores of Platt scaling (top) and t-scaling (bottom), comparing baselines and the proposed method. Importance weight are estimated using discriminator.}
\label{dann_mnist_usps}
\end{table}

\begin{table*}
\setlength\tabcolsep{2.5pt}
\begin{tabularx}{\textwidth}{@{} l l l l l l l l l l l l l  @{}}
\toprule
Method&Ar$\rightarrow$Cl&Ar$\rightarrow$Pr&Ar$\rightarrow$Rw&Cl$\rightarrow$Ar&Cl$\rightarrow$Pr&Cl$\rightarrow$Rw&Pr$\rightarrow$Ar&Pr$\rightarrow$Cl&Pr$\rightarrow$Rw&Rw$\rightarrow$Ar&Rw$\rightarrow$Cl&Rw$\rightarrow$Pr\\
\midrule
uncalibrated & 0.161 & 0.128 & 0.124 & 0.241 & 0.149 & 0.151 & 0.165 & 0.188 & 0.059 & 0.114 & 0.14  & 0.036 \\
unweighted   & 0.11  & 0.096 & 0.064 & 0.224 & 0.096 & 0.105 & 0.053 & 0.081 & 0.102 & 0.126 & 0.124 & 0.123 \\
Weighted & 0.115 & \textbf{0.086} & 0.486 & \textbf{0.14} & \textbf{0.074} & \textbf{0.071} & 0.116 & 0.177 & \textit{0.069} & \textbf{0.099} & 0.126 & \textit{0.058} \\
Using target & 0.07  & 0.099 & 0.045 & 0.1   & 0.104 & 0.029 & 0.068 & 0.073 & 0.045 & 0.035 & 0.059 & 0.04 \\ \hline \hline
unweighted   & 0.146 & 0.053 & 0.044 & 0.138 & 0.056 & 0.022 & 0.23  & 0.282 & 0.112 & 0.096 & 0.156 & 0.035 \\
Weighted &
  \textbf{0.117} &
  \textbf{0.046} &
  0.543 &
  \textbf{0.127} &
  \textbf{0.047} &
  \textbf{0.019} &
  \textit{0.215} &
  \textit{0.261} &
  \textit{0.084} &
  0.105 &
  0.166 &
  \textit{0.032} \\
Using target & 0.042 & 0.048 & 0.036 & 0.054 & 0.043 & 0.042 & 0.036 & 0.019 & 0.029 & 0.022 & 0.026 & 0.035 \\
\bottomrule
\end{tabularx}
\vspace{-0.1in}
\caption{Office-home, domain adapted using using DANN. ECE scores of Platt scaling (top) and t-scaling (bottom), comparing baselines and the proposed method. Importance weight are estimated using discriminator. }
\label{tab:office_home}
\end{table*}

\begin{table*}
\setlength\tabcolsep{2.5pt}
\begin{tabularx}{\textwidth}{@{} l l l l l l l l l l l l l  @{}}
\toprule
Method&Ar$\rightarrow$Cl&Ar$\rightarrow$Pr&Ar$\rightarrow$Rw&Cl$\rightarrow$Ar&Cl$\rightarrow$Pr&Cl$\rightarrow$Rw&Pr$\rightarrow$Ar&Pr$\rightarrow$Cl&Pr$\rightarrow$Rw&Rw$\rightarrow$Ar&Rw$\rightarrow$Cl&Rw$\rightarrow$Pr\\
\midrule
uncalibrated & 0     & 0     & 0     & 0     & 0     & 0     & 0     & 0     & 0     & 0     & 0     & 0     \\
unweighted   & 0     & 0     & 0.034 & 0     & 0.012 & 0.018 & 0.178 & 0     & 0.045 & 0.02  & 0     & 0     \\
weighted      & 0.001 & 0.002 & 0.009 & 0.001 & 0.002 & 0.002 & 0.001 & 0.001 & 0.002 & 0.003 & 0.001 & 0.002 \\
using target & 0     & 0     & 0     & 0.044 & 0.049 & 0.01  & 0     & 0.065 & 0     & 0     & 0.009 & 0  \\
\bottomrule
\end{tabularx}
\caption{Office-home, domain adapted using using CDAN. std values across 5-iterations in when platt scaling is used.}
\label{tab:x}
\end{table*}

\begin{table*}
\subfloat[0.55\linewidth][Office-31 dataset trained using pre-trained Resnet50.]{
    \setlength\tabcolsep{4pt}
    \begin{tabularx}{0.55\linewidth}{@{} l l l l l l l @{}}
    \toprule
    Method&A$\rightarrow$D&A$\rightarrow$W&D$\rightarrow$A&D$\rightarrow$W&W$\rightarrow$A&W$\rightarrow$D\\
    \midrule
    Unweighted&  0.023 & 0.032 & 0     & 0     & 0.088 & 0.081   \\
Weighted & 0.067 & 0.03  & 0.011 & 0.006 & 0.011 & 0.064   \\
Using target & 0     & 0.023 & 0.01  & 0.047 & 0     & 0   \\ 
    \bottomrule
    \end{tabularx}
    \label{tab:office_31}
}
\hfill
\subfloat[0.5\linewidth][Digits dataset, domain adapted using CDAN.]{
\setlength\tabcolsep{4pt}
    \begin{tabularx}{0.4\linewidth}{@{} l l l @{}}
    \toprule
    Method&U$\rightarrow$M&M$\rightarrow$U\\
    Unweighted & 0.117 & 0.145 \\
    Weighted & 0.056 & 0.039\\
    Using target & .001 & 0.005 \\
    \midrule
    \bottomrule
    \end{tabularx}
    \label{tab:digits}
}
%\vspace{-0.05in}
\caption{ECE std values on Platt scaling.}
\label{bigtable}
\end{table*}

\begin{table*}
\setlength\tabcolsep{2.5pt}
\begin{tabularx}{\textwidth}{@{} l l l l l l l l l l l l l  @{}}
\toprule
Method&Ar$\rightarrow$Cl&Ar$\rightarrow$Pr&Ar$\rightarrow$Rw&Cl$\rightarrow$Ar&Cl$\rightarrow$Pr&Cl$\rightarrow$Rw&Pr$\rightarrow$Ar&Pr$\rightarrow$Cl&Pr$\rightarrow$Rw&Rw$\rightarrow$Ar&Rw$\rightarrow$Cl&Rw$\rightarrow$Pr\\
\midrule
Weighted & 0.002 & 0.001 & 0.003 & 0.003 & 0.001 & 0.002 & 0.013 & 0.002 & 0.002 & 0.001 & 0.001 & 0.001 \\
\bottomrule
\end{tabularx}
\caption{Office-home, domain adapted using using CDAN.ECE  std values across 5-iterations in when temperature scaling is used.}
\label{tab:x}
\end{table*}

\begin{table*}
\subfloat[0.55\linewidth][Office-31 dataset trained using pre-trained Resnet50.]{
    \setlength\tabcolsep{4pt}
    \begin{tabularx}{0.55\linewidth}{@{} l l l l l l l @{}}
    \toprule
    Method&A$\rightarrow$D&A$\rightarrow$W&D$\rightarrow$A&D$\rightarrow$W&W$\rightarrow$A&W$\rightarrow$D\\
    \midrule
Weighted &  0.009 & 0.015 & 0.024 & 0.005 & 0.019 & 0.004 \\
    \bottomrule
    \end{tabularx}
    \label{tab:office_31}
}
\hfill
\subfloat[0.5\linewidth][Digits dataset, domain adapted using CDAN.]{
\setlength\tabcolsep{4pt}
    \begin{tabularx}{0.4\linewidth}{@{} l l l @{}}
    \toprule
    Method&U$\rightarrow$M&M$\rightarrow$U\\
    Weighted & 0.001 & 0.003 \\
    \bottomrule
    \end{tabularx}
    \label{tab:digits}
}
%\vspace{-0.05in}
\caption{ECE std values on temperature scaling.}
\label{bigtable}
\end{table*}

\begin{table*}
\subfloat[0.55\linewidth][Office-31 dataset trained using pre-trained Resnet50.]{
    \setlength\tabcolsep{4pt}
    \begin{tabularx}{0.55\linewidth}{@{} l l l l l l l @{}}
    \toprule
    Method&A$\rightarrow$D&A$\rightarrow$W&D$\rightarrow$A&D$\rightarrow$W&W$\rightarrow$A&W$\rightarrow$D\\
    \midrule
    uncalibrated & 0.782 & 0.746 & 0.623 & 0.897 & 0.64  & 0.963 \\
unweighted   & 0.783 & 0.731 & 0.532 & 0.858 & 0.629 & 0.965 \\
weighted     & 0.785 & 0.707 & 0.48  & 0.867 & 0.626 & 0.967 \\
using target & 0.839 & 0.848 & 0.731 & 0.965 & 0.732 & 0.983 \\
    \bottomrule
    \end{tabularx}
    \label{tab:office_31}
}
\hfill
\subfloat[0.5\linewidth][Digits dataset, domain adapted using CDAN.]{
\setlength\tabcolsep{4pt}
    \begin{tabularx}{0.4\linewidth}{@{} l l l @{}}
    \toprule
    Method&U$\rightarrow$M&M$\rightarrow$U\\
    \midrule
    uncalibrated & 0.525 & 0.667 \\
    unweighted & 0.521 & 0.546 \\
    weighted & 	0.518 & 0.617 \\
    using target &  0.685&  0.914 \\
    \bottomrule
    \end{tabularx}
    \label{tab:digits}
}
%\vspace{-0.05in}
\caption{Accuracy values on Platt scaling. t-scaling keeps accuracy constant. std values less than 0.006.}
\label{bigtable}
\end{table*}

\begin{table*}
\setlength\tabcolsep{2.5pt}
\begin{tabularx}{\textwidth}{@{} l l l l l l l l l l l l l  @{}}
\toprule
Method&Ar$\rightarrow$Cl&Ar$\rightarrow$Pr&Ar$\rightarrow$Rw&Cl$\rightarrow$Ar&Cl$\rightarrow$Pr&Cl$\rightarrow$Rw&Pr$\rightarrow$Ar&Pr$\rightarrow$Cl&Pr$\rightarrow$Rw&Rw$\rightarrow$Ar&Rw$\rightarrow$Cl&Rw$\rightarrow$Pr\\
\midrule
uncalibrated & 0.263 & 0.373 & 0.537 & 0.316 & 0.414 & 0.433 & 0.328 & 0.229 & 0.518 & 0.444 & 0.293 & 0.607 \\
unweighted   & 0.254 & 0.345 & 0.524 & 0.317 & 0.412 & 0.432 & 0.307 & 0.211 & 0.511 & 0.444 & 0.28  & 0.607 \\
weighted      & 0.245 & 0.311 & 0.504 & 0.291 & 0.409 & 0.427 & 0.298 & 0.204 & 0.512 & 0.433 & 0.27  & 0.597 \\
using target & 0.31  & 0.497 & 0.574 & 0.323 & 0.523 & 0.489 & 0.349 & 0.273 & 0.577 & 0.451 & 0.338 & 0.653 \\
\bottomrule
\end{tabularx}
\caption{Office-home, domain adapted using using CDAN. Accuracy values when platt scaling is used. Temperature scaling keeps the accuracy constant. Std deviation values are less than0.007}
\label{tab:x}
\end{table*}
